# Supplementary material for: Analyzing Inverse Problems with Invertible Neural Networks
Source: arXiv:1808.04730 source file (2019-02-06)
Supplement: Supplementary file 1 [file supplement_removed_experiments.tex]

\section{Artificial data -- complex forward process}

In the main paper, we showed an artificial example in 2D. 
The complexity of that example lies in the shape of the prior, whereas the forward process is almost trivial.
In the following, we present an additional example, where the forward process is more complex, and continuous as opposed to discrete.
To construct this example, we begin with a standard normal distribution, which is then distorted and projected onto a line.
This line is then again distorted to form a one-dimensional curve in 2D $\y$-space, shown in the top left panel of Fig.~\ref{fig:compl_forward}. 
The three points marked on the curve map to the sub-manifolds in $\x$-space indicated in the bottom right panel.

As shown in the top right, the INN solves the inverse problem correctly, using a latent dimensionality of $\mathrm{dim}(z) = 1$.
For comparison, we also train an MMD-GAN with an equal number of parameters, which is also able to generate correct solutions.
Both the dropout samping method and a cGAN did not converge to satisfactory solutions.

\begin{figure}[h!]
\begin{center}
\includegraphics{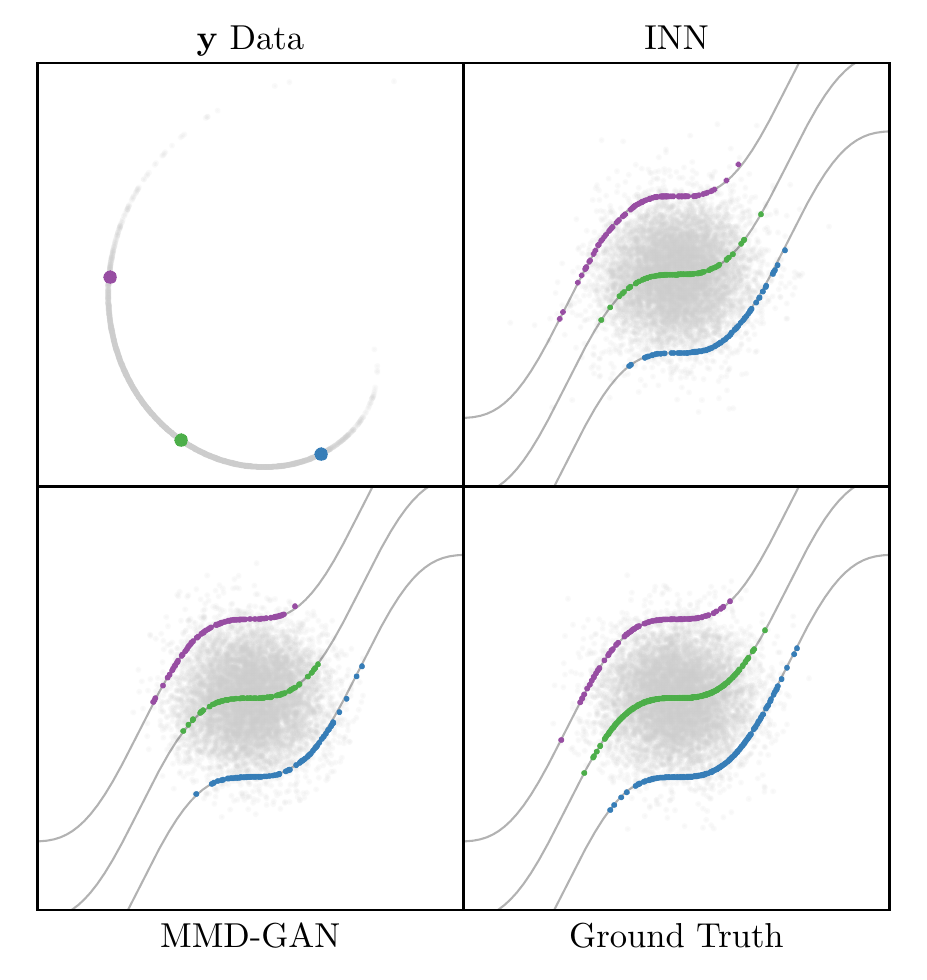}
\end{center}
\caption{In clockwise order: $\y$-space of the artificial problem, $\x$-space with solution manifolds, MMD-GAN results, INN results}
\label{fig:compl_forward}
\end{figure}

\section{Artificial Data -- High-dimensional Distributions}

In addition to the low-dimensional examples shown so far, we demonstrate an artificial example with a higher dimensionality.
Hereby, we construct a Gaussian mixture model with 32 mixture components in 128-dimensional space to supply the hidden variables $\x$. 
The mixture components all have the same variance, and are scattered randomly around the origin, such that each mode has some overlap with the others. 
The forward process is given by 16 projections along random directions, producing the observations $\y$.
This is in contrast to the example used in the main paper, where there was no overlap between mixture components, and the forward process was defined simply by mode labelling.

We now train four networks on this task: (i) INN, (ii) a Monte Carlo dropout network with learned aleatoric error term, (iii) a simple feed forward network for point estimates, and (iv) a generator with MMD loss on this problem -- each with an approximately equal number of parameters in an attempt to ensure similar expressive power.
We could not reach meaningful convergence on this task with a cGAN, despite our best efforts.
We compare these methods in various ways, summarized in the figures below.

Firstly, we analytically compute the linear subspace in the $\x$-domain that contains correct solutions to the inverse problem. 
For each possible solution sampled from the posterior of a given method, we can then calculate the closest point in this subspace.
This gives us a measure of how far a method's solutions lie from the manifold of true solutions. 
This is tallied over many validation samples, and shown as a histogram in Fig.~\ref{fig:subspace_dist_hist}, top. 
We find that the INN produces by far the most accurate results. 
As the forward process is a matrix multiplication and therefore trivial to learn, the inverse is correct to a high accuracy.
The point estimate method follows close behind, with the other methods performing significantly worse.
Surprisingly, the generator trained with MMD performs the worst by far, although it visually worked very well in the low-dimensional artificial example.

Secondly, we pick a single validation data point, and sample from the estimated posterior of the sampling-based methods.
We then perform principal component analysis (PCA) on these samples, the singular values of which are shown in Fig.~\ref{fig:pca}, middle.
We know that the posterior has $128-16 = 112$ dimensions, therefore it should only possess 112 non-zero singular values. 
We see that the INN learns to approximate this well, while the generator output collapses to a single point for a fixed $\y$, and the Monte Carlo dropout network samples solutions from the entire 128 dimensions, as it is not able to separate the correlated axes.

Lastly, we compare the quality of the priors produced when accumulating the network outputs over all validation samples, shown in Fig.~\ref{fig:likelihood_hist}, bottom. 
Naturally, the point estimates lie in extremely high likelihood regions, while the INN and Monte Carlo dropout network match the prior adequately.
In fact, the dropout network matches the distribution better, as the prior will be composed of Gaussians by construction, whereas the shape has to be learned by the INN. The generator + MMD architecture is also centered around the correct region, but the distribution is much too broad, with both implausibly high- and low-likelihood solutions occurring.

\begin{figure}[h!]
\begin{center}
\includegraphics{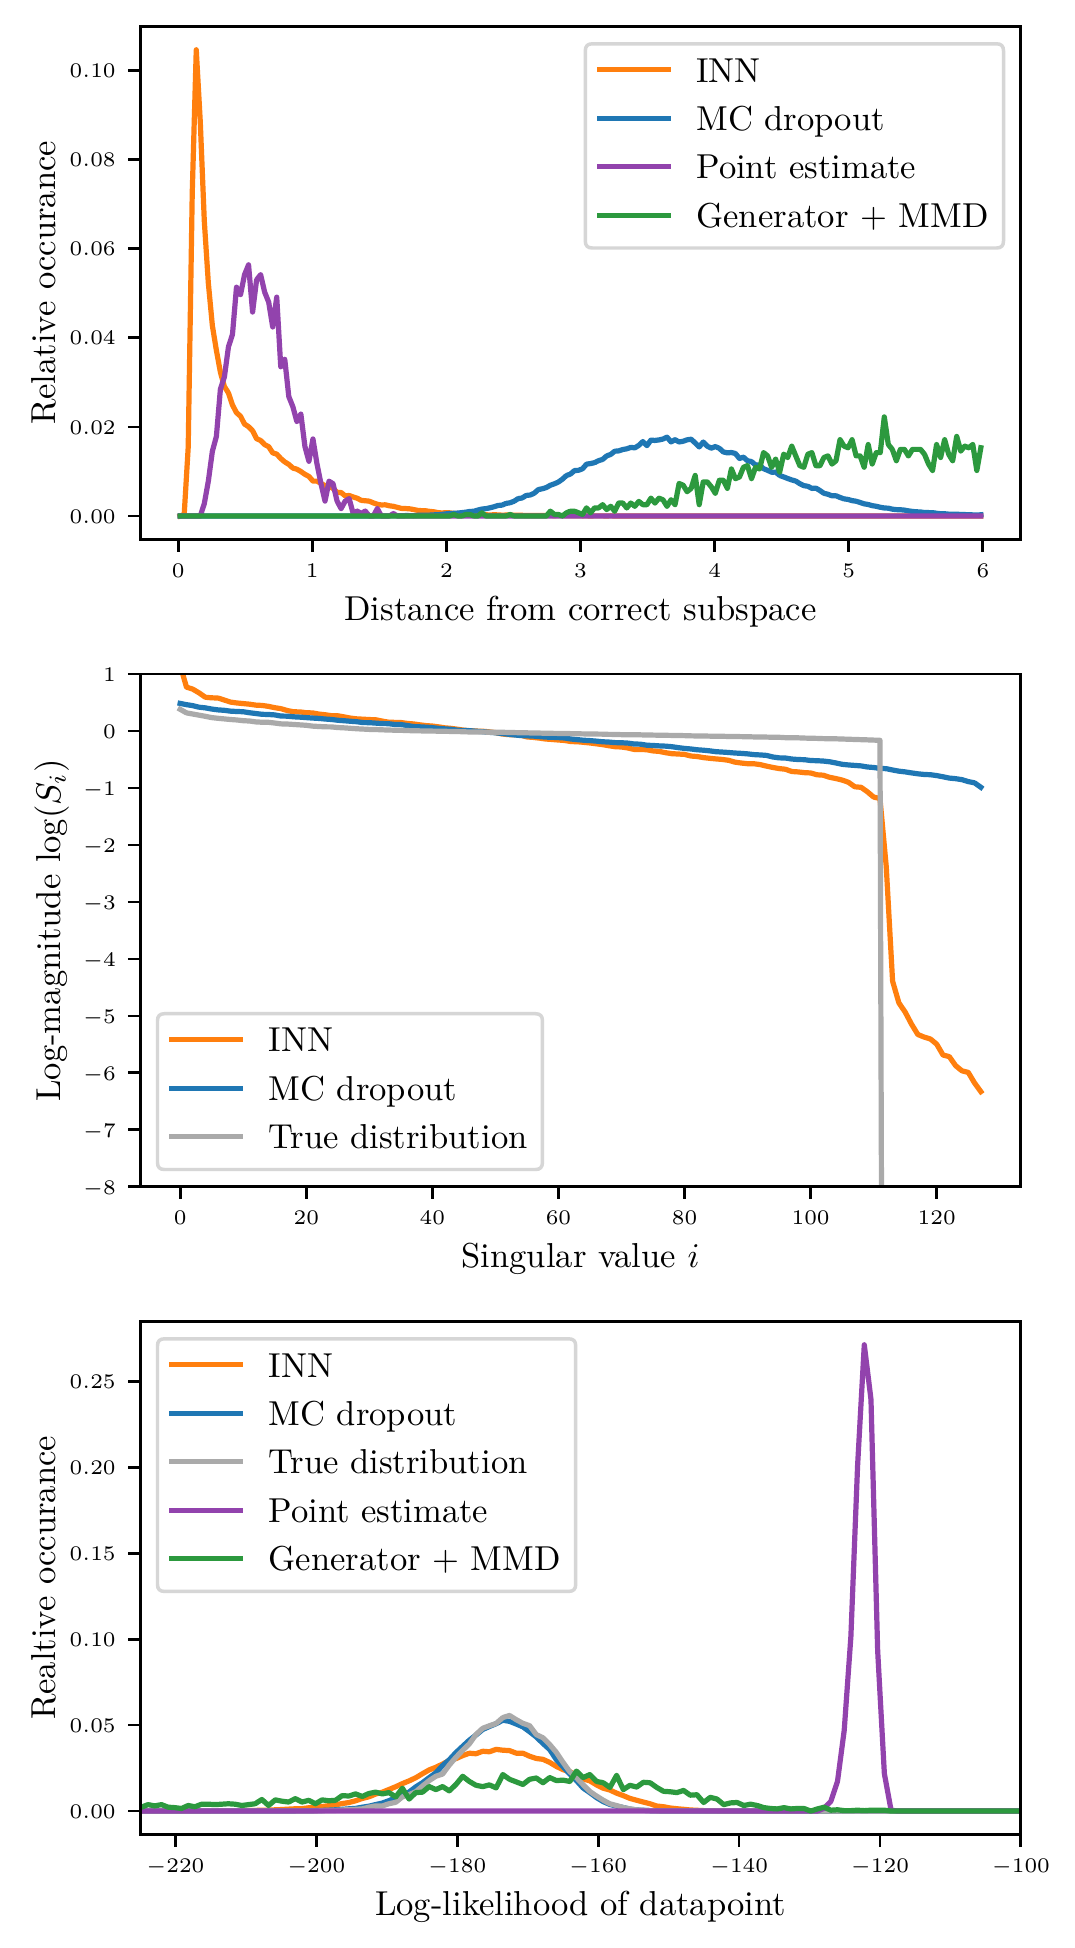}
\end{center}
\caption{\textit{From top to bottom:}
(i) Distribution of $\ltwo$-errors between the solutions to the inverse problem given by each method and the closest point in the subspace of true solutions.
(ii) Magnitude of the singular values of samples conditioned on a single observation $\y$.
(iii) Distribution of likelihoods of the outputs of each method compared to the true prior $p(\x)$.}
\label{fig:pca}
\label{fig:subspace_dist_hist}
\label{fig:likelihood_hist}
\end{figure}

\FloatBarrier
\section{Calibration curve for tissue parameter estimation}
\todo[inline]{update the calibration curve with other methods}

\begin{figure}[h!]
\begin{center}
\includegraphics{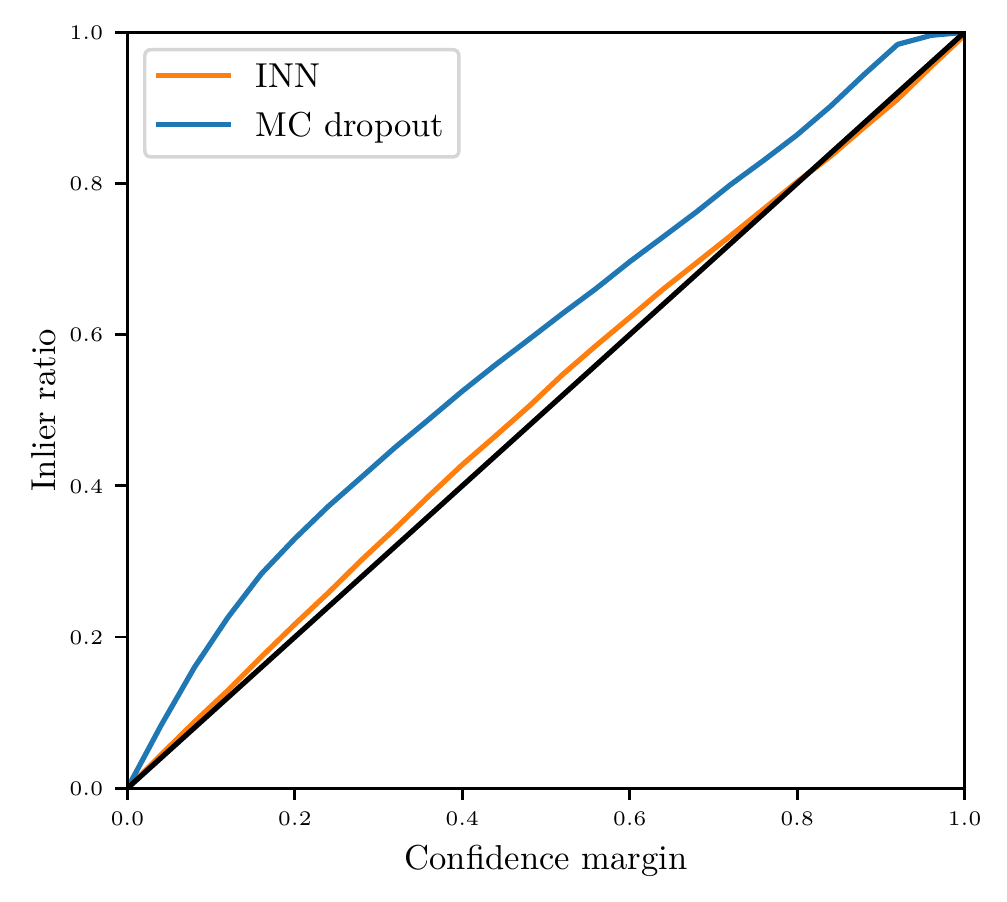}
\end{center}
\caption{The full calibration curve, used to calculate the median calibration error in the main paper. We see that the curve of the INN is considerably closer to the true (\emph{black}) curve.}
\end{figure}

% \subsection{High-dimensional artificial data}
% \paragraph{INN:} 5 invertible blocks, with 2 fully connected layers and a leaky ReLU activation in the intermediate layer. Adam optimizer, learning rate decay from $2\cdot10^{-4}$ to $2\cdot10^{-6}$, batch size 200. No zero padding, inverse multiquadratic kernel with $\alpha = 100$.
% \paragraph{Monte Carlo dropout/point estimate:} 7 fully connected layers, ReLU activiations, Adam optimizer, learning rate decay from $10^{-3}$ to $10^{-6}$, batch size 200.
% \paragraph{Generator with MMD:}  7 fully connected layers, leaky ReLU activiations, Adam optimizer, learning rate decay from $10^{-3}$ to $10^{-6}$, batch size 256, inverse multiquadratic kernel, $\alpha = 100$.

%\todo[inline]{update/remove in case MCMC/BOLFI/etc is used}
%\section{Approximate Bayesian Computation algorithm}
%\begin{algorithm}[H]
%\SetAlgoLined
%\KwResult{Set of samples from the posterior $S_\y = \left\{ \x_k \mid \x_k \sim p(\x|\y)\right\}$}
% Training set $S_\text{train}$, number of samples $N_\text{samples}$, Gaussian noise in $\y$ with width $\sigma_\y$.\\
% Initialize $S_\y \gets \{\}$\;
% \For{$1 \le i \le N_\text{samples}$}{
%  Draw with replacement $(\x_i, \y_i) \in S_\text{train}$\;
%  Compute $\rho_i = \exp\left(- \frac{\| \y_i - \y\|^2}{2\sigma_\y^2}\right)$\;
%  Draw $r_i \sim \text{Unif}(0,1)$\;
%  \If{$\rho_i \ge r_i$}{
%   $S_\y \gets S_\y \cup \{\x_i\}$\;
%  }
% }
% \caption{Approximate Bayesian Computation using a discrete training set}
%\end{algorithm}

\FloatBarrier
